# Supplementary material for: HyperLLaVA: Dynamic Visual and Language Expert Tuning for Multimodal Large Language Models
Source: arXiv:2403.13447 source file (2024-03-20)
Supplement: Supplementary file 2 [file appendix.tex]

% \documentclass[10pt,onecolumn,letterpaper]{article}
% \usepackage{times}
% \usepackage{latexsym}
% \usepackage[T1]{fontenc}
% \usepackage[utf8]{inputenc}

% \usepackage{float}
% \usepackage{newfloat}
% \usepackage{multirow}
% \usepackage{makecell}
% \usepackage{xcolor}         % colors
% \usepackage{colortbl}
% \usepackage{dsfont}
% \usepackage{amsmath}
% % \usepackage{align}
% \usepackage{enumitem}

% % \usepackage{multirow}
% \usepackage[normalem]{ulem}
% \useunder{\uline}{\ul}{}

% \definecolor{myyellow}{rgb}{1,1, 0.6}
% \definecolor{myorange}{rgb}{1, 0.8, 0.6}
% \definecolor{myred}{rgb}{1, 0.6, 0.6}
% \definecolor{second}{HTML}{FFDAB9}
% \definecolor{best}{HTML}{FFC1C1}
% \usepackage{multirow}
% \usepackage{colortbl}
% \usepackage[normalem]{ulem}
% \usepackage{bbding}
% \useunder{\uline}{\ul}{}
% \usepackage{stackrel}
% \usepackage{todonotes}
% \usepackage{booktabs}
% \newcommand*{\method}{HyperLLaVA}
% % \pagestyle{plain}

% \renewcommand{\todo}[1]{\iffalse #1 \fi{\color{blue} \textbf{[TODO]}}}

% \begin{document}
% %Is Multi-Stage Learning Necessary?
% \title{ Appendix}
% \maketitle


% This is the Appendix for ``Revisiting the Domain Shift and Sample Uncertainty in Multi-source Active Domain Transfer''. Table~\ref{tab:abb} summarizes the abbreviations and the symbols used in the main body of our paper. 

% \begin{table}[h]
% \begin{center}
% \captionsetup{font={small,stretch=1.25}, labelfont={bf}}
% \caption{ Abbreviations and symbols used in the main paper.}
%  \renewcommand{\arraystretch}{1.2}
% \resizebox{0.7\textwidth}{!}
%  {
%   \begin{tabular}{c||c }
%    \toprule[1.5pt]
%    \textbf{Abbreviation/Symbol} & \textbf{Meaning}\\
%    \hline
%    \hline
%    & \underline{\emph{Abbreviation}}\\
%      Domain Adaptation&DA\\
%       Unsupervised Domain Adaptation&UDA\\
%       Active Domain Adaptation&ADA\\
%    Multi-source Domain Adaptation &  MSDA\\
%     Multi-source Active Domain Adaptation &  MADA\\
%     Source Domain &  $\mathcal{D}_s$\\
%     Multi-source  Domain &  $\{\mathcal{D}_{s,i}\}^M_{i=1}$\\
%     Target Domain &  $\mathcal{D}_t$\\
%      \hline
%    \hline
%      & \underline{\emph{Symbol in Algorithm}}\\
%        Detective  & Dynamic integrated uncertainty valuation framework\\
%        $\mathcal{M}(\cdot;(\Theta_{{m}},\Theta_{{a}}))$  & MADA Model\\
%        $\mathcal{M}(\cdot;\Theta_{{m}})$  & Multi-domain Adaptation Model\\
%        $\mathcal{M}(\cdot;\Theta_{{a}})$  & Active Learning Model\\
%        $Dir(\cdot)$  & Dirichlet Distribution\\
%        $H(\cdot)$  & Shannon Entropy\\
%        $\mathcal{U}_{dom}$  & Domain Uncertainty \\
%        $\mathcal{U}_{pre}$  & Predictive Uncertainty\\
%        $\mathcal{U}_{ins}$  & Integrated Uncertainty\\
%        $\mathcal{D}_{con}$  & Contextual Diversity\\
%        UDN  & Universal Dynamic Network\\
%       IUS  & Integrated Uncertainty Selector\\
%         CDC  & Contextual Diversity Calculator\\
%         $\mathcal{L}_{mar}$  & Marginal Likelihood  Loss\\
%         $\mathcal{L}_{kl}$  & KL-divergence Loss\\
%    \toprule[1.5pt]
%   \end{tabular}
%   }
%   \label{tab:abb}
% \end{center}
% \end{table}






% This appendix is organized as follows: 


% \begin{itemize}

% \item Section ~\ref{sec:1} provides the method details of proposed \method{}, including Integrated Uncertainty Selector (IUS) and Contextual Diversity Calculator (CDC).


% \item Section ~\ref{sec:2} reports more experimental settings of baselines, implementation details and training process of \method{}.

% \item Section ~\ref{sec:3} shows the additional experiments on the \texttt{Office-Home}~\cite{venkateswara2017deep} and \texttt{Digits-five}~\cite{nguyen2021most} dataset to further verify the effectiveness of \method{}.

% \item Section ~\ref{sec:4} lists the limitations of this paper.
% \end{itemize}



% \subsection{HyperLLaVA Training}
% We optimize the output of \method{} through a generative loss in an auto-regressive manner. Given an image and text, \method{} generates the output sequence $R = [r_1, r_2, \cdots, r_k]$ by progressively
% generating each element, where K = P + D represents the
% length of the output sequence. The formula is:
% \begin{align}
% \label{eq:adapter}
% \begin{gathered}
% L=-\sum_{i=1}^K(R^{P+i}|V,T^{[:i-1]})
% \end{gathered}
% \end{align}

% \noindent\textbf{Implementation Details.}  
% In the training of the \method{}, we utilize the ADAMW optimizer, adapting hyperparameters to cater to the specific requirements of each phase. For the feature alignment stage, parameters are set as \(B=32\), \(Lr=0.001\), while for the visual instruction tuning stage, we adjust the parameters to \(B=16\), \(Lr=0.00002\). The configuration for the ADAMW optimizer incorporates the following settings: \(\boldsymbol{\beta} = (0.9, 0.999)\), \(\varepsilon = 1 \times 10^{-8}\), and $W_d$ = 0.0, ensuring a bespoke optimization strategy that effectively addresses the unique demands of each training phase.

% We train our model following the same training process as LLaVA-1.5. The process includes two stages: (1) feature alignment stage: use 558K subset of the LAION-CC-SBU dataset to connect a frozen pretrained vision encoder to a frozen LLM; (2) visual instruction tuning stage: use 150K GPT-generated multimodal instruction-following data, plus around 515K VQA data from academic-oriented tasks, to teach the model to follow multimodal instructions.







% {\small
% % \bibliographystyle{ieee_fullname}
% \bibliography{custom}
% }

% \end{document}
